# Supplementary material for: Homophily based on few attributes can impede structural balance
Source: arXiv:2001.06573 source file (2020-01-18)
Supplement: Supplementary file 1 [file sm-18-1.pdf]

# Supplemental Material - Homophily based on few attributes can impede structural balance

Piotr J Górski, Klavdiya Bochenina, Janusz A. Hołyst, Raissa M. D'Souza

January 18, 2020

## 1 Asymptotic analytical solutions

### 1.1 Using exact transition probabilities

As mentioned in the main paper, knowing all transition probabilities one can calculate the exact measures of balanced states, for instance for $(N = 3, G = 3)$ the paradise probability is as follows:

$$P_P(p) = \frac{25 + 37p}{32(5 - p)} \tag{S1}$$

Figure S1 shows a transition diagram for a single triad of agents possessing 3 attributes each $(N = 3, G = 3)$. In this simple example there are only 4 types of different systems. Similar diagrams for more complicated cases would require more system types. With increasing $G$ one needs to consider different kinds (in terms of distances between nodes) of triads of different type. For $G = 3$ there is only one possible triad $\Delta_1$ and one possible triad $\Delta_3$. For $G = 5$ there are two kinds of triad $\Delta_1$. From $G = 7$ one needs to take also into account different kinds of triad $\Delta_3$. With $N > 3$ even more complicated transitions arise, as types of balanced triads have to be considered. In such a case it would be necessary to consider distances between all the agents or, equivalently, position of agents in the Hamming space. The number of needed types grows very quickly with $N$ and $G$. That is why calculating exact relations for systems with larger values of $N$ and $G$ is unfeasible.

### 1.2 Notation and introductory analysis

Let us use the following symbols (the first three follow [1]):

- $n_k$ — density of triads $\Delta_k$,
- $\rho$ — density of positive links,
- $n_k^{\pm}$ — density of triads $\Delta_k$ attached to a positive $(n_k^+)$ or to a negative link $(n_k^-)$,

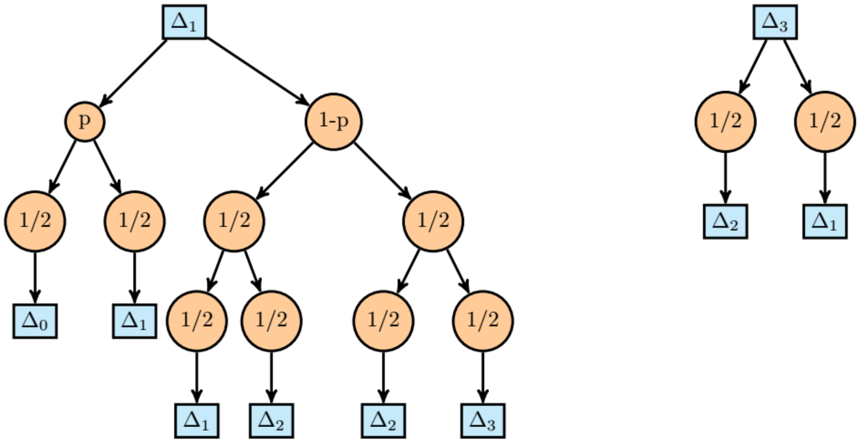


FIG. S1: Transition diagram for $N = 3, G = 3$. $\Delta_k$ corresponds to a triad with $k$ negative links. Values in circles correspond to probabilities.

- $x_{ij}$ — edge weight which is a transformed Hamming distance between nodes $i$ and $j$. If Hamming distance $d_{ij}$ between $i$ and $j$ is the number of differences in attributes of these nodes normalized by the total number of attributes $G$, then the edge weight is defined as $x_{ij} = 0.5 - d_{ij}$. The value of $x_{ij}$ may vary from $-0.5$ to $0.5$. Positive (negative) values of $x_{ij}$ correspond to the positive (negative) link. Further in the text, when it does not lead to a confusion, the indices $(ij)$ are neglected and the weight is denoted simply as $x$.

Above variables are intertwined:

$$n_k^+ = \frac{(3-k)n_k}{3\rho} \tag{S2}$$

$$n_k^- = \frac{kn_k}{3(1-\rho)} \tag{S3}$$

We assume large numbers $N$ and $G$. As a consequence of large number of nodes $N$, two randomly chosen triads are uncorrelated. Thus, one can calculate density $n_k$ using positive $\rho$ and negative $(1-\rho)$ link densities: $n_0 = \rho^3$, $n_1 = 3\rho^2(1-\rho)$, $n_2 = 3\rho(1-\rho)^2$ and $n_3 = (1-\rho)^3$. These relations are not fulfilled when the balanced, non-paradise state is reached.

## 1.3 Jump probabilities in random walk approximation

Figure S2 visualizes the idea of the proposed random walk for edge weights.

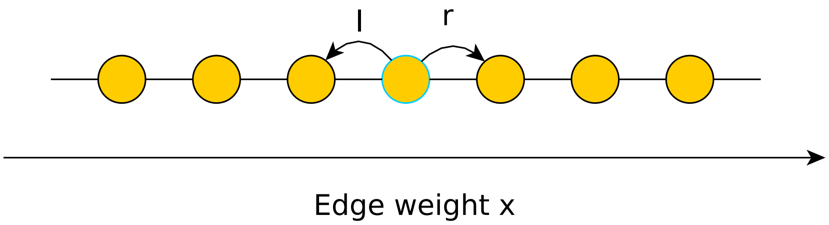


FIG. S2: Schematic picture of Random Walk approximation for changes of edge weights. In each update a walker (weight value) may move to the right, to the left or stay with corresponding probabilities: $r$, $l$ and $1-(r+l)$. The values $r$ and $l$ are not constant but are dependent on edge weight $x$.

Jump probabilities in this random walk can be expressed by the following general probabilistic relations:

$$r \equiv P(r) = P(r|AC)P(AC) + P(r|IC)P(IC) \tag{S4}$$

$$l \equiv P(l) = P(l|AC)P(AC) + P(l|IC)P(IC) \tag{S5}$$

Accidental change (AC) for a positive or a negative link is caused by the involvement of this link in unbalanced triads (for a positive link only in $\Delta_1$ and for a negative link both in $\Delta_1$ or $\Delta_3$) or due to being adjacent to any of unbalanced triads. This is described by following equations where $P(AC|x > 0) = a_+$ and $P(AC|x < 0) = a_-$:

$$a_+\binom{N}{3} = \underline{\underline{n_1^+(N-2)\frac{1+p}{4}}} \qquad + \qquad 2\binom{N-2}{2}\frac{n_1+n_3}{3} \tag{S6}$$

$$a_-\binom{N}{3} = \underline{\underline{n_1^-(N-2)\frac{1-p}{2}}} + \underline{\frac{n_3^-(N-2)}{3}} + 2\binom{N-2}{2}\frac{n_1+n_3}{3} \tag{S7}$$

On the other hand, incidental changes (ICs) are caused only by link's involvement in unbalanced triads. Let us denote probabilities of the IC, $P(IC|x > 0)$ and $P(IC|x < 0)$, as $i_+$ and $i_-$, respectively. Then:

$$i_+\binom{N}{3} = \underline{\underline{n_1^+(N-2)\frac{1-p}{2}}} \tag{S8}$$

$$i_-\binom{N}{3} = \underline{\underline{n_1^-(N-2)p}} + \underline{\frac{n_3^-(N-2)}{3}} \tag{S9}$$

In Eqs. (S6-S9) the double-underlined and underlined terms correspond to the involvement of this link in triads $\Delta_1$ and $\Delta_3$, respectively and the remaining term corresponds to the case when the link is adjacent to an unbalanced triad.

The conditional probabilities of an accidental jump (e.g. $P(r|AC)$) can be easily calculated using combinatorial methods: $P(r|AC) = d = 0.5 - x$ and

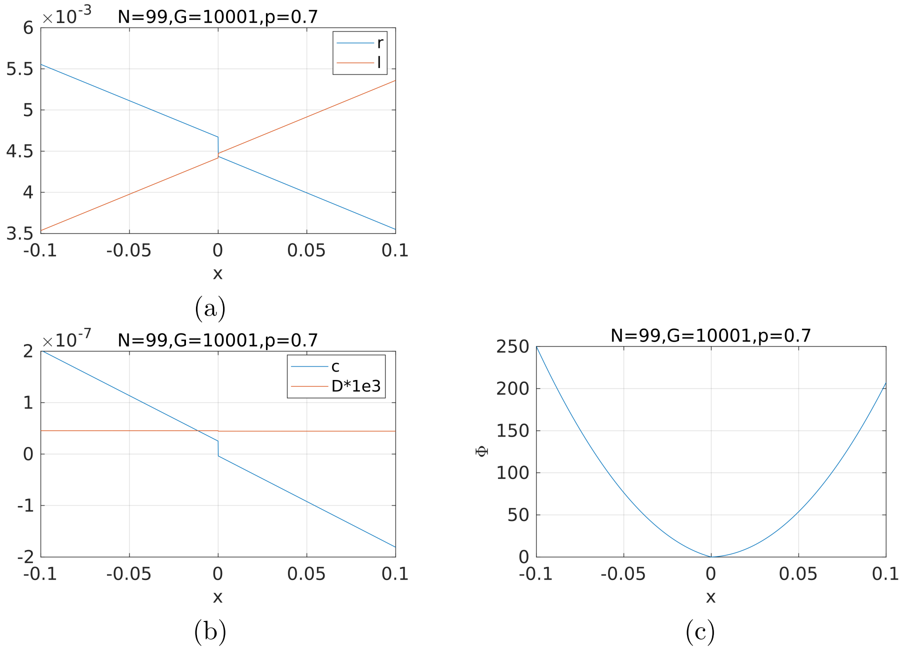


FIG. S3: Analytical results for the system with numbers of nodes $N = 99$, number of attributes $G = 10001$ and consensus parameter $p = 0.7$. Panel (a) shows Random Walk probabilities of 'jumping right' $r$ and 'jumping left' $l$ as a function of link weight $x$. Panel (b) shows drift $c(x)$ and diffusion $D(x)$ coefficients of the Fokker-Planck equation and panel (c) shows the potential $\Phi(x)$ in the quasi-stationary state.

$P(l|AC) = 1 - d = 0.5 + x$. Conditional incidental jump probabilities are as follows: $P(r|IC) = \begin{cases} 0 & \text{for } x > 0 \\ 1 & \text{for } x < 0 \end{cases}$ and $P(l|IC) = \begin{cases} 1 & \text{for } x > 0 \\ 0 & \text{for } x < 0 \end{cases}$. Taking above analysis together, equations for jump probabilities can be written as [the Eqs. (1-2) from the main text]:

$$r(x) = \begin{cases} (0.5 - x)a_+ & \text{for } x > 0 \\ (0.5 - x)a_- + i_- & \text{for } x < 0 \end{cases} \tag{S10}$$

$$l(x) = \begin{cases} (0.5 + x)a_+ + i_+ & \text{for } x > 0 \\ (0.5 + x)a_- & \text{for } x < 0 \end{cases} \tag{S11}$$

The example probabilities for a system ($N = 99$, $G = 10001$ and $p = 0.7$) are shown in Fig. S3a.

## 1.4 Fokker-Planck equation

Assuming an infinite number of possible states ($G \to \infty$) one can calculate the quasi-stationary solution of the Random Walk process using Fokker-Planck equations (FPE).

$$\frac{\partial W(x,t)}{\partial t} = -\frac{\partial}{\partial x}\big(c(x)W(x,t)\big) + \frac{\partial^2}{\partial x^2}\big(D(x)W(x,t)\big), \tag{S12}$$

with drift $c$ and diffusion $D$ as [2, 3]: $c(x) = \frac{\Delta x}{\Delta t}(r-l)$ and $D(x) = \frac{(\Delta x)^2}{2\Delta t}(r+l)$, where $\Delta x$ can be identified with $1/G$ and $\Delta t$ — with a single update. Thus, one can calculate [4] the potential $\phi(x)$ and the quasi-stationary solution $W_{st}(x) \propto e^{-\phi(x)}$.

$$\phi(x) = \frac{2G}{a_\pm + i_\pm}\Big(a_\pm x^2 + i_\pm |x|\Big), \tag{S13}$$

where $a_+$ and $i_+$ are used for positive links and $a_-$ and $i_-$ when $x < 0$. See Figs. S3b and S3c for exemplary $c(x)$, $D(x)$ and $\Phi(x)$.

Equation S13 allows us to derive an analytical equation for the quasi-stationary values of positive link density $\rho$, as: $\rho = \int_{x>0} W_{st}(x)dx$.

Let us denote $W_{st}^\pm$ as integrals of $\exp\Big(-\phi(x)\Big)$ over positive or negative domain. Then we have:

$$W_{st}^\pm = \exp\Big(\frac{C_\pm^2}{2}\frac{G}{N^2}\Big)\sqrt{\frac{a_\pm + i_\pm}{a_\pm}}\,\Phi\Big(-C_\pm\frac{\sqrt{G}}{N}\Big)\sqrt{\frac{\pi}{2G}}, \tag{S14}$$

where $C_\pm = N\frac{i_\pm}{\sqrt{a_\pm(a_\pm + i_\pm)}}$ and $\Phi$ is a standard normal cumulative distribution function.

Thus, we find:

$$\rho = \int_{x>0} W_{st}(x)dx = \frac{W_{st}^+}{W_{st}^+ + W_{st}^-} \tag{S15}$$

which leads to:

$$\rho = \left(1 + \exp\Big(\frac{C_-^2 - C_+^2}{2}\frac{G}{N^2}\Big)\sqrt{\frac{a_- + i_-}{a_-}}\sqrt{\frac{a_+}{a_+ + i_+}}\frac{\Phi_-}{\Phi_+}\right)^{-1}, \tag{S16}$$

where $\Phi_\pm = \Phi\Big(-C_\pm\frac{\sqrt{G}}{N}\Big)$.

In the equation above both sides are functions of $\rho$. Thus, for any specific case it is possible to solve it using graphical method. Simpler solutions arise in the thermodynamical limit (see Sec. 1.6).

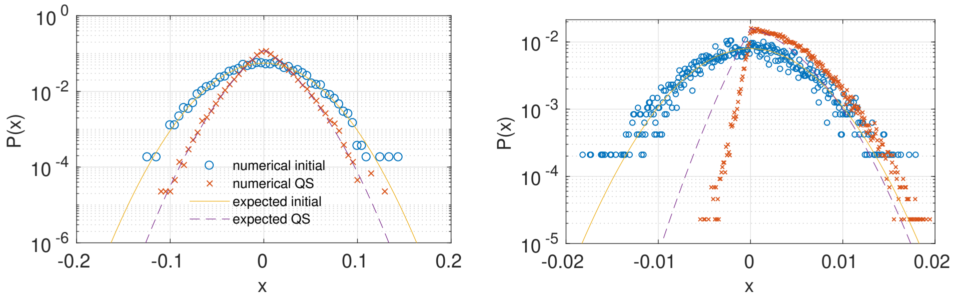


(a) $N = 11, G = 205, p = 0.4$ (b) $N = 99, G = 10001, p = 0.7$

FIG. S4: Comparison between analytical and numerical initial and quasi-stationary (QS) distributions for two different systems. Analytical and numerical results are very close in panel (a), whereas in panel (b) for the QS case there is some discrepancy. The legend for both panels is given in panel (a).

## 1.5 Link weight distribution

The initial link weight distribution follows a Binomial distribution, which for sufficiently large number of attributes can be approximated with a normal distribution $\mathcal{N}\Big(\mu = 0, \sigma^2 = \dfrac{1}{4G}\Big)$. The analysis of the previous section lets us calculate the stationary link weight distribution $W_{st}(x)$.

Figure S4 compares the analytical approximations of initial and stationary distributions with distributions received from numerical simulations. For the chosen systems the analytical stationary results show the distribution of the quasi-stationary state. Data from numerical simulations correspond also to such a state, although a balanced state is always eventually reached.

Obtained quasi-stationary distributions are much more centered around the polarity threshold $x = 0$ than the initial distributions. In other words, links in the quasi-stationary state are more likely to change their polarity than in the random initial case. The reason for this is as follows. Both ICs and ACs processes move a link's weight $x$ towards the threshold, because IC can flip the polarity of the given link to make the triad balanced and for the ACs the reason is related to combinatorics (see conditional probabilities of an accidental jump in Sec. 1.3). The analytical approximation for the quasi-stationary distribution is much better for smaller values of $p$. The discrepancy in Fig. S4b is related to the discrepancy also observed in the Fig. 2 in the main text.

## 1.6 Thermodynamical limit

Following Sec. 1.4 we, first, check whether the paradise ($\rho = 1$) is a valid solution. In the thermodynamical limit the following equations hold:

$$\frac{a_+ + i_+}{a_+} \xrightarrow{N\to\infty} 1$$
$$\frac{a_- + i_-}{a_-} \xrightarrow{N\to\infty} \frac{1+p}{1-p}$$
$$C_+ \xrightarrow{N\to\infty} 2(1-p)$$
$$C_- \xrightarrow{N\to\infty} N\frac{2p}{\sqrt{1-p^2}}$$

Thus, the solution for density of positive links $\rho$ given by Eq. (S16) transforms in the thermodynamical limit into $\rho = 1$ with the exception of the case $p \sim 1/N$ (because then $C_+ \sim C_-$). This shows that as long as $p \gg 1/N$ the paradise state is a possible solution.

Now, outside the residuum, *i.e.*, for $\rho < 1$, let us use the above mentioned relation $n_k(\rho)$ and the following variables: $\tilde{C}_+ = 3\rho(1-p)$, $\tilde{C}_- = \frac{3\rho^2 p + (1-\rho)^2}{1-\rho}$, $C_\rho = 3\rho^2 + (1-\rho)^2$. In the thermodynamical limit it is possible to write $C_\pm = \frac{\tilde{C}_\pm}{C_\rho}$. With $\rho < 1$ the relations $\frac{a_\pm + i_\pm}{a_\pm} \xrightarrow{N\to\infty} 1$ are fulfilled and the solution (S16) for the positive link density can be written as:

$$\rho = \frac{\Phi_+}{\Phi_+ + \exp\Big(\frac{G}{N^2}\frac{C_-^2 - C_+^2}{2}\Big)\Phi_-}. \tag{S17}$$

Let us assume the following relation: $G = O(N^\gamma)$. Then, dependent on the exponent $\gamma$ the recurring term $G/N^2$ will either go to infinity ($\gamma > 2$), be a constant ($\gamma = 2$) or become 0 ($\gamma < 2$). The analysis for $\gamma \neq 2$ is given in the main text.

## 1.7 Transition analysis for $\gamma = 2$

If $\gamma = 2$, then the system reaches an intermediate asymptotic solution. Assuming $G = b^2N^2$, then $N$ and $G$ cancel out from (S17). It is possible to show that depending on the parameter $b$ there exists a transition point $p^*$ such that for $p > p^*$ the only solution is $\rho = 1$. Let us write the r.h.s. of Eq. (S17) as $f(\rho, p, b)$. One can show that $f(\rho = 0, p, b) > 0$ and for reasonable $p$ it was earlier shown that paradise is a solution, *i.e.*, $f(\rho = 1, p, b) = 1$. Thus, for given $p$ a quasi-stationary solution does not exist if $\forall\rho\ \frac{d}{d\rho}f(\rho, p, b) \leq 1$, because such a condition means that l.h.s. and r.h.s. of (S17) will cross only once in $\rho = 1$. The exact value of $p^*$ can be obtained from the following condition: $\lim_{\rho\to 1^-}\frac{d}{d\rho}f(\rho, p, b) = 1$, which allows to obtain:

$$\frac{1}{\sqrt{2\pi}}\exp\Big(-\frac{1}{2}b^2(1-p^*)^2\Big) = bp^*\Phi\Big(-b(1-p^*)\Big) \tag{S18}$$

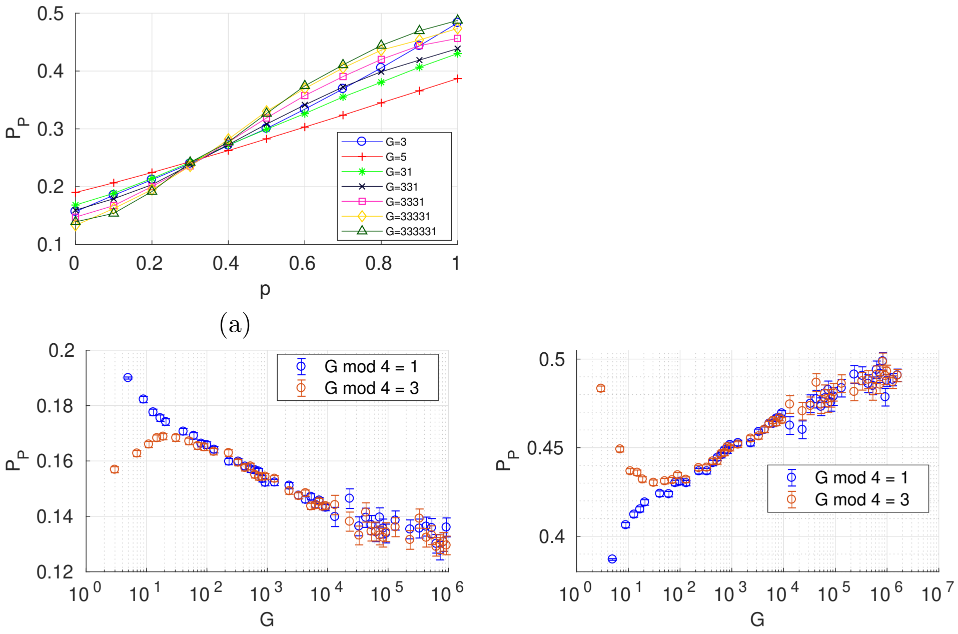


(a)

(b) $p = 0$

(c) $p = 1$

FIG. S5: No transition in the case of systems with only one triad. Probability of reaching paradise $P_P$ as a function of parameter $p$ for several numbers of attributes $G$. Panel (a) shows $P_P(p)$ for different values of $G$. Panels (b) and (c) show the $P_P(G)$ for $p = 0$ and $p = 1$, respectively. The error bars represent approx. 68% confidence intervals. If not shown, the error bars are smaller than marker size.

As $p^*$ cannot be larger than 1, for $\gamma = 2$ a transition exists as long as $b \geq \sqrt{\frac{2}{\pi}}$.

## 2 No transition in 3-node network

First, let us focus on numerical results of a 3-node system. Figure S5 shows the probability of reaching a paradise for different values of parameter $p$ and different number of attributes $G$. The increase of $P_P(p)$ is approximately linear for small $G$ and of higher order for large $G$ (Fig. S5a). Panels (b) and (c) show the relation $P_P(G)$ for $p = 0$ and $p = 1$. Those panels show two different curves for $G \mod 4 = 1$ and $G \mod 4 = 3$. The significant difference between these curves can be observed for small values of $G$ ($G < 100$). For this range the increase of $G$ does not lead to monotonic change of $P_P(p)$ curve. With the increase of number of attributes two series ($G \mod 4 = \pm 1$) converge.

Second, let us derive the probability of having a paradise for infinite number

of attributes. Assuming random initial conditions characterized in the main paper, the probability of paradise formula is as follows:

$$P_P(p) = \frac{1}{8} + P_{\Delta_1 \to \Delta_0}(p)\frac{3}{8} \tag{S19}$$

Equations (8-9) in our main paper describe changes of links' weights in a triad of type $\Delta_1$. The solution of Eqs. (8-9) is as follows:

$$\begin{aligned} x_-(t, p < 1) &= \frac{p}{1-p} - \frac{E_-}{1-p}\exp\Big(-(1-p)t\Big) \\ x_-(t, p = 1) &= t + \tilde{E}_- \\ x_+(t) &= -\frac{1-p}{1+p} + \frac{2E_+}{1+p}\exp\Big(-\frac{1+p}{2}t\Big), \end{aligned} \tag{S20}$$

where $E_-$, $\tilde{E}_-$ and $E_+$ are constants.

From these solutions it is possible to predict the output for the cases of $p = 0$ and $p = 1$. For $p = 0$ the negative link's weights and for $p = 1$ the positive links' weights will never cross the threshold point 0: $x_-(p = 0) = x_+(p = 1) \xrightarrow{t\to\infty} 0$. It means that when $p = 0$ ($p = 1$) a triad of type $\Delta_1$ will always turn into $\Delta_2$ ($\Delta_0$). Thus, knowing initial triad distributions we obtain $P_P(p = 0) = 0.125$ and $P_P(p = 1) = 0.5$. To obtain the probability $P_P$ for intermediate values of $p$ one needs to calculate the system probability density functions (PDFs) of escape times $t_\pm$ (moments when when variables $x_\pm$ cross 0).

$$\begin{aligned} t_- &= \frac{1}{1-p}\ln\Big(\frac{E_-}{p}\Big) \\ t_+ &= \frac{2}{1+p}\ln\Big(\frac{2E_+}{1-p}\Big) \end{aligned} \tag{S21}$$

The PDF of an initial link weight between two nodes [*i.e.*, $x(t = 0)$] can be approximated using the normal distribution: $\mathcal{N}\Big(\mu = 0, \sigma^2 = \frac{1}{4G}\Big)$. Knowing the sign of the link lets us define the *half-normal* distribution denoted as $\mathcal{N}_{0.5}(\mu, \sigma^2)$:

$$f\Big(x|\mathcal{N}_{0.5}(\mu,\sigma^2)\Big) = \begin{cases} 2f\Big(x|\mathcal{N}(\mu,\sigma^2)\Big) & \text{when} \quad x > \mu \\ 0 & \text{when} \quad x < \mu \end{cases} \tag{S22}$$

The weight of a random positive link is described with $\mathcal{N}_{0.5}(0, \frac{1}{4G})$. The weight of a random negative link is described with $\mathcal{N}_{-0.5}(0, \frac{1}{4G})$, where a minus signifies that in Eq. (S22) the relations are reverse, *i.e.*, $f\Big(x|\mathcal{N}_{-0.5}(\mu,\sigma^2)\Big) = 0$ when $x > \mu$. This allows calculating the PDFs of constants $E_-$ and $E_+$ as

$\mathcal{N}_{0.5}\Big(p, \dfrac{1}{4G}(1-p)^2\Big)$ and $\mathcal{N}_{0.5}\Big(\dfrac{1-p}{2}, \dfrac{1}{4G}(\dfrac{1+p}{2})^2\Big)$, which leads to PDFs of escape times $t_{\pm}$ (for $t > 0$):

$$f_{t_-}(t) = \frac{4\sqrt{G}}{\sqrt{2\pi}} \exp\Big(-2G\Big(\frac{p}{1-p}(e^{(1-p)t}-1)\Big)^2\Big)pe^{(1-p)t} \tag{S23}$$
$$f_{t_+}(t) = \frac{4\sqrt{G}}{\sqrt{2\pi}} \exp\Big(-2G\Big(\frac{1-p}{1+p}(e^{\frac{1+p}{2}t}-1)\Big)^2\Big)\frac{1-p}{2}e^{\frac{1+p}{2}t}$$

Probability of a change $\Delta_1 \to \Delta_0$ is equivalent to calculating the probability that a negative link will be first to change polarity, *i.e.*, the probability $P(\tau_-^3 < \tau_+^1, \tau_+^2)$, where $\tau_{\pm}^l$ are random variables given by PDFs $f_{t_\pm}(t)$ ($l$ denotes link number in a single triad):

$$\begin{aligned} P_{\Delta_1\to\Delta_0} &= P(\tau_-^3 < \tau_+^1, \tau_+^2) = P\Big(\tau_-^3 < \min(\tau_+^1, \tau_+^2)\Big) = \\ &= \int_{-\infty}^{+\infty}\Big(\int_{\tau_-^3}^{+\infty} f_{\min(\tau_+^1,\tau_+^2)}(\tau_+)d\tau_+\Big) f_{t_-}(\tau_-^3)d\tau_-^3 = \\ &= \int_{-\infty}^{+\infty}\Big(1 - F_{\min(\tau_+^1,\tau_+^2)}(\tau_-^3)\Big) f_{t_-}(\tau_-^3)d\tau_-^3, \end{aligned} \tag{S24}$$

where $f_{\min(\tau_+^1,\tau_+^2)}(\tau_+)$ is the PDF of a minimum of two random variables given by $f_{t_+}$ and the capital $F$ signifies the corresponding cumulative density function (CDF). One can show the following relation for a CDF of a minimum of two random variables from the same distribution:

$$F_{\min(\tau_+^1,\tau_+^2)}(t) = 1 - \big(1 - F_{t_+}(t)\big)^2 \tag{S25}$$

After some transformations, we obtained the final relation:

$$P_{\Delta_1\to\Delta_0}(p) = 4\int_{-\infty}^{+\infty}\Big(1 - \Phi\big(h(\tau)\big)\Big)^2 f_{t_-}(\tau)d\tau, \tag{S26}$$

where $h(\tau) = 2\sqrt{G}\dfrac{1-p}{1+p}\Bigg(\exp\Big(\dfrac{1+p}{2}\tau\Big) - 1\Bigg)$ and $\Phi$ is a standard normal CDF.

# 3 Systems with set number of attributes

Systems with agents possessing a single attribute are a special case of the presented model. Such systems do not exhibit any evolution as they are straightforwardly balanced. Nodes with $a_1^1 = +1$ have positive ties towards similar nodes and negative to those with $a_1^1 = -1$. That is why the observed measures do not depend on parameter $p$. One can calculate the values of those measures:

$$P_P(G=1) = 2^{-(N-1)} \tag{S27}$$

$$\rho(G=1) = 0.5 \tag{S28}$$

Figure S6 presents results for systems with $G = 3$, $G = 5$ and $G = 7$ attributes. Results of observed measures (paradise probability $P_P$ and density of positive links in a balanced final state $\rho_{bal}$) for different number of attributes are qualitatively similar. The value of consensus probability $p$ matters less for small $N$. In such systems, the fate of a system is highly related to the initial state, which is close to being balanced. When the number of nodes increases different curves diverge. Density $\rho_{bal}$ changes with $N$ as follows: for small values of $p$, $\rho_{bal}$ changes towards $\rho_{bal} = 0.5$, whereas for higher $p$, $\rho_{bal}$ decreases. When $N \approx 20$, $\rho_{bal}$ reaches an approximately constant value. On the other hand the probability $P_P$ seems not to decrease only for $p = 1$. With $G > 3$, for $p < 1$ it may initially increase for small $N$, but with approx. constant $\rho_{bal}$ ($N > 20$), probability $P_P$ starts falling. The explanation of this relationship is as follows. The value of positive link density in the balanced state is directly related to the size of the final larger group (for instance with $\rho_{bal} \approx 0.5$ most of the final states consist of two groups of approximately same size). With a given mean value of $\rho_{bal}$ the deviation of ratio of nodes in the larger group remains approximately constant. It means that for a larger number of agents the probability that all of them form a paradise state is decreasing.

# 4 Systems with set number of nodes

Figure S7 shows the results (paradise probability $P_P$ and density of positive links in a balanced final state $\rho_{bal}$) for systems with a set number of nodes (from 5 to 9) and varying number of attributes. These results can be also compared with the results for $N = 3$ (Fig. S5) and for $N = 11$ (Fig.5b in the main paper). With more agents, the probability that randomly chosen initial conditions are close to a balanced state decreases. The outcome of a system far away from being balanced is greatly dependent on value of $p$. The transition from a balanced state with two approximately equal-sized groups (corresponding to $\rho_{bal} \approx 0.5$) to (almost) a paradise (corresponding to $\rho_{bal} \approx 1$) is observed for medium values of $p$. The transition is becoming steeper when number of agents and number of attributes increase. The presented results indicate that for $p > 0.5$ and for a large number of attributes the system nearly always reaches the paradise state.

# 5 Invariant features

We hypothesize that for a system with a given number of nodes $N$ there exists a value of parameter $p$ equal to $\tilde{p} = 1/3$, where all considered measures (e.g. probability of paradise $P_P$, density of positive links, both, $\rho$ and $\rho_{bal}$) do not depend on the number of attributes $G$. If this hypothesis is true, the exact

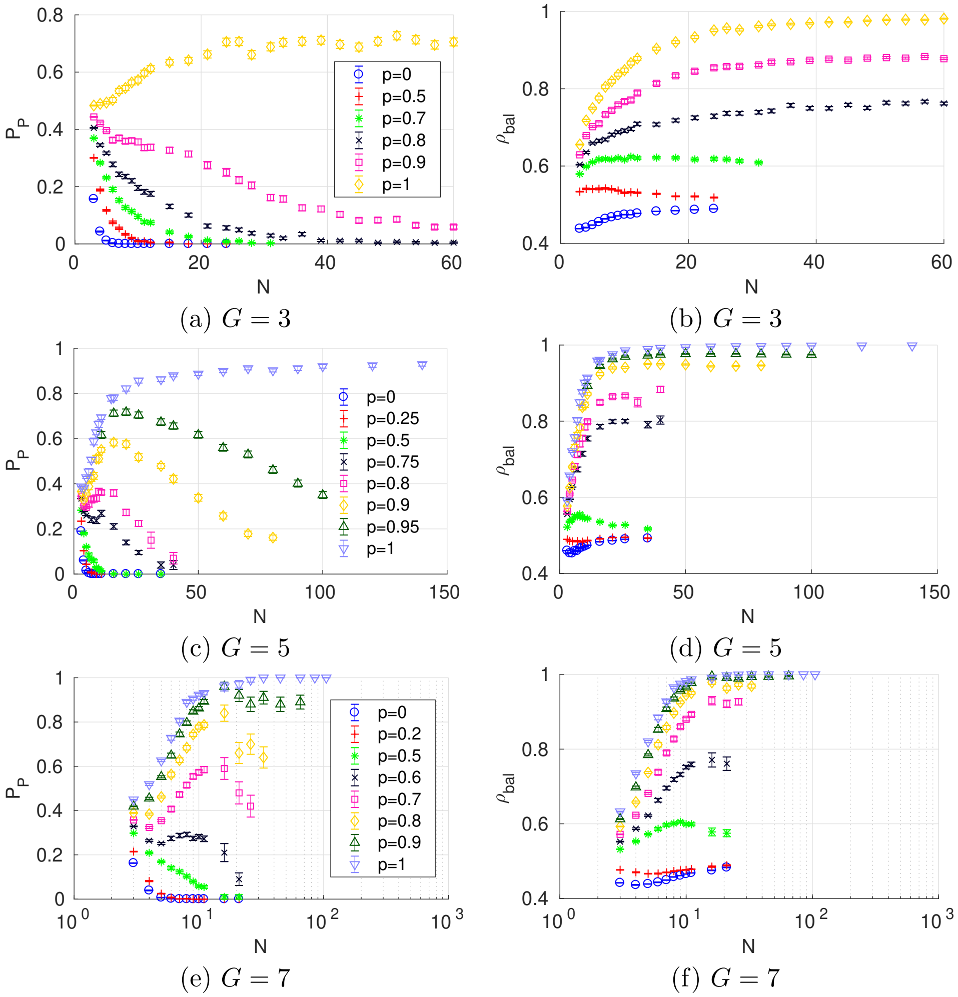


(a) $G = 3$ (b) $G = 3$

(c) $G = 5$ (d) $G = 5$

(e) $G = 7$ (f) $G = 7$

FIG. S6: Changes of paradise probability $P_P$ and density of positive links in final, balanced state $\rho_{bal}$ for systems with varying number of agents $N$ and number of attributes $G$ set to 3, 5, or 7. The relevant legends are displayed in the left column.

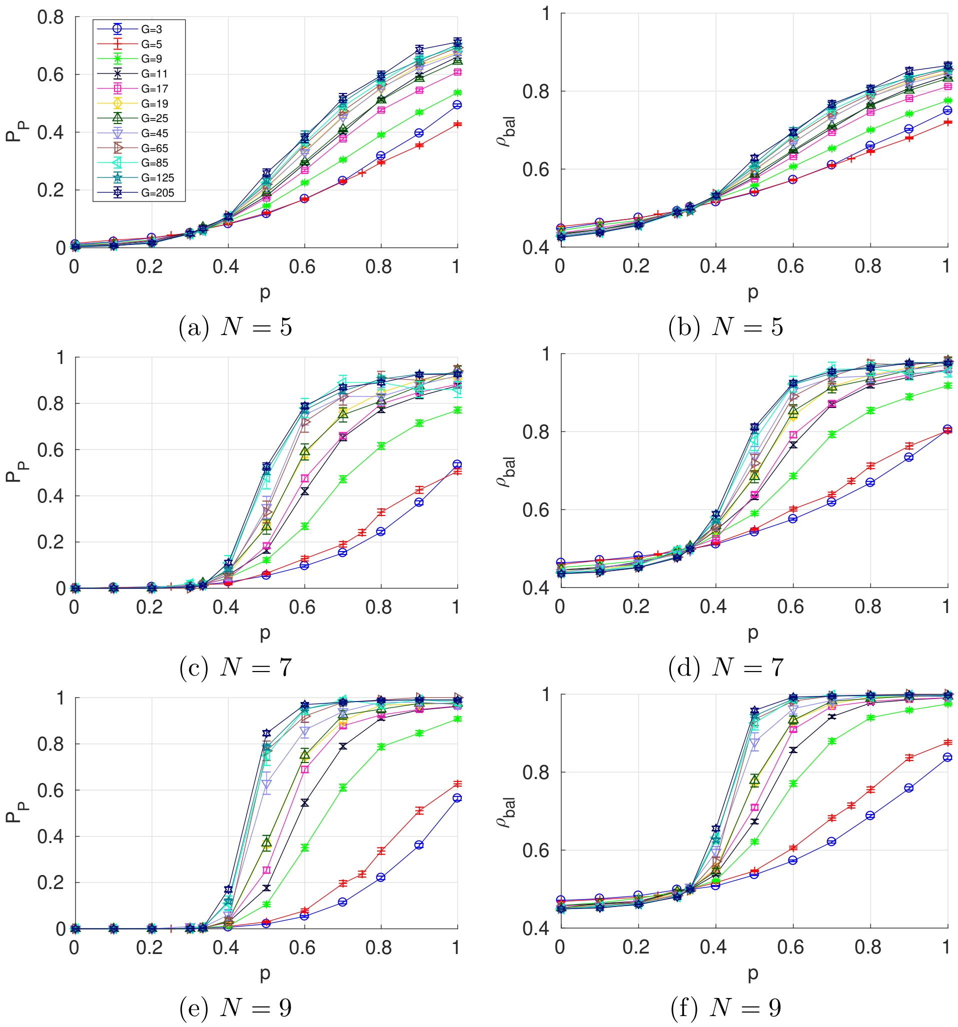


(a) $N = 5$ (b) $N = 5$

(c) $N = 7$ (d) $N = 7$

(e) $N = 9$ (f) $N = 9$

FIG. S7: Changes of paradise probability $P_P$ and density of positive links in final, balanced state $\rho_{bal}$ for systems with varying number of attributes $G$ and number of agents $N$ set to 5, 7 or 9. The relevant legends are displayed in panel (a).

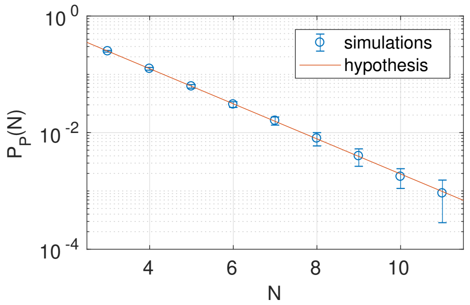


(a) $N = 5$

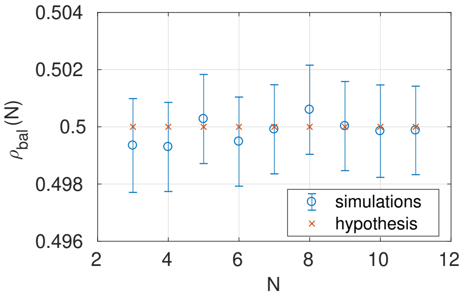


(b) $N = 5$

FIG. S8: Comparison between values predicted by the hypothesis and obtained in the numerical simulations averaged over systems with varying number of attributes $G > 1$ for $\tilde{p} = 1/3$ of (a) paradise probability $P_P$ and (b) positive link density in the final, balanced state $\rho_{bal}$. The hypothesis that for $\tilde{p}$ these measures do not depend on the number of attributes $G$ cannot be rejected.

values of $P_P(\tilde{p})$ and $\rho(\tilde{p})$ can be calculated from a system of agents with a single attribute (S27)-(S28): $P_P(\tilde{p}) = 0.25$ and $\rho = 0.5$.

We cannot prove this hypothesis analytically, but we note that it is confirmed by several numerical and analytical observations:

- numerical results for the density of positive links in a quasi-stationary state (Fig. 2);
- analytical asymptotic results for $\gamma > 2$, $\gamma = 2$ and $\gamma < 2$ (Figs. 2, 3 and 4a);
- numerical results for small and large $G$ for $N = 3$ (Fig. 5a and Fig. S5);
- analytical results for $N = 3$ and $G \to \infty$ (Fig. 5a). Also, one can show that PDFs of times $t_{0.5}$ in Eq. (S23) are identical for $p = 1/3$. In the system with three random variables governed by the same PDF a chosen variable is the smallest in $1/3$ cases, which gives $P_P(G \to \infty, \tilde{p}) = \frac{1}{8} + \frac{1}{3} \cdot \frac{3}{8} = \frac{1}{4}$;
- numerical results for small $N$ (Figs. S7 and S8)

Figure S8 shows the comparison between the numerical and expected results for $p = 1/3$. We performed double-sided tests. We calculated p-values of the hypotheses for each measure ($P_P$ and $\rho$) and for each $N$ separately. Using the Holm-Bonferroni correction we cannot reject any of the hypotheses keeping the error rate at level 0.05.

# References


[1] Tibor Antal, Paul L Krapivsky, and Sidney Redner. Dynamics of social balance on networks. *Physical Review E*, 72(3):36121, 2005.

[2] Eli Ben-Naim, Pavel L Krapivsky, and Sidney Redner. Fundamental kinetic processes. *Boston University, Boston, MA*, 2008.

[3] Edward A. Codling, Michael J. Plank, and Simon Benhamou. Random walk models in biology. *Journal of the Royal Society Interface*, 5(25):813–834, 2008.

[4] Hannes Risken. Fokker-planck equation. In *The Fokker-Planck Equation*. Springer, 1996.
